# Supplementary material for: Are Tabular Foundation Models Robust to Realistic Query Distribution Shifts in Microbiome Data?
Source: arXiv:2606.24995 source file (2026-06-23)
Supplement: Supplementary file 1 [file main_supplementary.tex]

\documentclass[runningheads]{llncs}
\usepackage[T1]{fontenc}
\usepackage{graphicx}
\usepackage{booktabs}
\usepackage{xcolor}
\usepackage{algorithm}
\usepackage{algpseudocode}
\usepackage{amsmath}
\usepackage{amssymb}
\usepackage{dsfont}
\usepackage{cleveref}
\usepackage{subcaption}
\usepackage{caption}
\usepackage[misc]{ifsym}

\graphicspath{{supplementary_material/images/}}

\begin{document}
\appendix
\input{appendix}

\clearpage
\bibliographystyle{splncs04}
\bibliography{biblio}
\end{document}
